# Supplementary material for: Follower Agnostic Methods for Stackelberg Games
Source: arXiv:2302.01421 source file (2024-03-27)
Supplement: Supplementary file 1 [file NumericsAppendix.tex]

% \begin{figure}
%     \centering
%     \includegraphics[width=0.9\textwidth]{Figures/WheatstoneLatest/PriceTrajectories.png}
%     \caption{Caption}
%     \label{fig:enter-label}
% \end{figure}
